# Supplementary material for: Linear instability in thermally-stratified quasi-Keplerian flows
Source: arXiv:2410.04913 ancillary file (2024-10-07)
Supplement: Supplementary file 1 [file Supplementary_material_3rdrevision_v1.pdf]

This document was prepared using the LaTeX style file belonging to J. Fluid Mech.

# Supplementary material for the main paper titled "Linear instability in thermally-stratified quasi-Keplerian flows"

**Dongdong Wan[1], Rikhi Bose[2], Mengqi Zhang[1,3]† and Xiaojue Zhu[2]‡**

[1]Department of Mechanical Engineering, National University of Singapore, 9 Engineering Drive 1, 117575, Singapore

[2]Max Planck Institute for Solar System Research, 37077 Göttingen, Germany

[3]NUS Research Institute (NUSRI) in Suzhou, No. 377 Linquan Street, Suzhou, Jiangsu, 215123, China

CONTENTS

**1. Numerical validation and convergence** 1
**2. Transformation required for the comparison with Deguchi (2017)** 1
**3. Mode structure similarities between high and low Taylor numbers** 3
**4. Mode patterns of the linear instabilities at high azimuthal wavenumbers** 3
**5. Linear instability in an extreme case at** $(\eta, Pr, Ri)$=$(0.05, 10^{-7}, 10^{-7})$ 4

## 1. Numerical validation and convergence

To validate our code, we conducted comparisons with data from Deguchi (2017) pertaining to isothermal TC flows. Encouragingly, our results exhibit a good agreement with theirs, as summarised in table 1.

We have demonstrated the convergence of the eigenspectra to graphical accuracy in figure 2 of the main paper. Here, we additionally provide a mesh-independence study of the unstable modes and list their eigenvalues in table 2 for further comparison. It is evident that the eigenvalues converge well with increased spatial resolution $N$, and numerical accuracy can be achieved up to about 10 significant digits for $N \geqslant 21$. Calculations at relatively extreme parameters, such as those in section 4.3 of the main paper, can be computationally intensive and require much higher resolutions up to $N = 401$ to achieve good convergence.

## 2. Transformation required for the comparison with Deguchi (2017)

In section 1 of this document, we have validated our eigenvalue computation by comparing with the results in Deguchi (2017). Since these two studies use different non-dimensionalisation methods, control parameters, and frame of references, transformation is needed for the comparison. We derive the transformation formulae for this purpose as follows.

† Email address for correspondence: mpezmq@nus.edu.sg
‡ Email address for correspondence: zhux@mps.mpg.de

| | Deguchi (2017) | The present |
|---|---|---|
| Growth rate | 9.1339 | 9.133636 |
| Frequency | 259281.859 | 259281.85942 |

Table 1: Validation of the present code for the computation of the leading eigenvalue of the isothermal Taylor-Couette flow at $\eta = 5/7$, $q \approx -17.9181$, $Ta \approx 3.09415 \times 10^{14}$, $m = 2$ and $k = 1.504$. These parameters are transformed from those given in table I of Deguchi (2017). Note that our direct computation in a rotating frame of reference yields an eigenvalue of $-0.783737509764 + 0.000000640898i$. This value, once transformed back to the fixed frame of reference, corresponds to the entry shown in the table. The transformation method is described in section 2 of this document.

| $N$ | The leading eigenvalue | The second eigenvalue |
|---|---|---|
| 7 | $0 + 0.535463407121511i$ | $0 + 0.113639548363407i$ |
| 11 | $0 + 0.527625869174870i$ | $0 + 0.097706821117094i$ |
| 21 | $0 + 0.527583254541696i$ | $0 + 0.097656247419922i$ |
| 51 | $0 + 0.527583254484749i$ | $0 + 0.097656247384773i$ |
| 151 | $0 + 0.527583254487419i$ | $0 + 0.097656247405420i$ |

Table 2: Convergence of the eigenvalues of the two unstable modes shown in figure 2($a$) of the main paper for the Keplerian case at $\eta = 0.3$, $Pr = 0.7$, $Ri = 0.1$ and $Ta = 10^6$; the axial wavenumber is $k = 5$ and the azimuthal wavenumber is $m = 0$. Zero real parts of the eigenvalues indicate stationary waves. For comparison, the eigenvalue of the most unstable mode for $(k, m) = (0, 1)$ is $0.4881230309 + 0.1325868404i$; those for $(k, m) = (5, 1)$ are $0.5637733964 + 0.3658303193i$ and $0.4038967359 + 0.1297377720i$.

The first step is to transform the parameters ($Re_i = \omega_i^* r_i^* d^*/\nu^*, Re_o = \omega_o^* r_o^* d^*/\nu^*$) used in Deguchi (2017) to our parameters ($Ta, q$). Note that both of these two studies use the cylinder gap ($d^* = r_o^* - r_i^*$) as the characteristic length scale for non-dimensionalisation and the definitions of the radius ratio $\eta$ are the same as well. Thus, no transformation is needed for the wavenumbers $(m, k)$. For Taylor number,

$$\begin{aligned} Ta &= \frac{(1+\eta)^4}{64\eta^2} \frac{d^{*2}(r_i^* + r_o^*)^2(\omega_i^* - \omega_o^*)^2}{\nu^{*2}} \\ &= \frac{(1+\eta)^4}{64\eta^2} \frac{d^{*2}(r_i d^* + r_o d^*)^2 \left[(Re_i \nu^*)/(r_i^* d^*) - (Re_o \nu^*)/(r_o^* d^*)\right]^2}{\nu^{*2}} \\ &= \frac{(1+\eta)^4}{64\eta^2} \left(\frac{Re_i}{r_i} - \frac{Re_o}{r_o}\right)^2 (r_i + r_o)^2. \end{aligned} \tag{2.1}$$

Note that the non-dimensional $r_i$ and $r_o$ are given by $\eta$ in Eq. (2.2$b$) of the main paper. For the rotation exponent parameter,

$$\eta^q = \frac{\omega_o}{\omega_i} = \frac{\omega_o^*}{\omega_i^*} = \frac{(Re_o \nu^*)/(r_o^* d^*)}{(Re_i \nu^*)/(r_i^* d^*)} = \frac{Re_o \eta}{Re_i}. \tag{2.2}$$

The second step is to transform the eigenvalue directly obtained from our code at $(q, Ta, k, m)$, which is in a frame of reference rotating with the angular frequency of the outer cylinder $\omega_o^*$, to a fixed frame of reference as in Deguchi (2017). In the normal mode assumption Eq. (2.8) of the main paper, the complex exponential under the rotating frame

of reference is in the form of $\exp(-i\omega t + im\theta)$ where we ignore the $ikz$ term as the rotating frame of reference does not move in the $z$ direction. The complex exponential under a fixed frame of reference takes the form of $\exp(-i\hat{\omega}t + im\hat{\theta})$. These two exponentials are related as

$$\exp(-i\hat{\omega}t+im\hat{\theta}) = \exp[-i\hat{\omega}t+im(\theta+\omega_o t)] = \exp[(-i\hat{\omega}+im\omega_o)t+im\theta] = \exp(-i\omega t+im\theta), \tag{2.3}$$

where the last equality is due to the fact that these two different exponentials represent the same wave component viewed in different frame of references. Then we have

$$-i\hat{\omega} + im\omega_o = -i\omega \quad \rightarrow \quad \hat{\omega} = \omega + m\omega_o. \tag{2.4}$$

It should be noted that these derivations are for non-dimensional quantities. Here, the non-dimensional angular frequency of the outer rotating cylinder can be calculated based on the non-dimensionalisation described in section 2.1 of the main paper as

$$\omega_o = \frac{d^*}{U^*}\omega_o^* = \frac{d^*\omega_o^*}{|\omega_i^* - \omega_o^*| r_i^*} = \frac{1}{2Ro} \tag{2.5}$$

where Rossby number $Ro$ is a function of the radius ratio $\eta$ and the rotation exponent parameter $q$ defined in Eq. (2.4) of the main paper.

The third step is to further transform the complex frequency $\hat{\omega}$ in the fixed frame of reference to the complex growth rate $\hat{\sigma}$ defined in Deguchi (2017). This transformation is necessary because different non-dimensionalisation methods are used in these two studies. Specifically, the time scale chosen by Deguchi (2017) is $d^{*2}/\nu^*$. Therefore, to have the dimensional quantities (marked with asterisk $^*$) equal as

$$-i\hat{\omega}^* = \sigma^*, \tag{2.6}$$

we should have

$$-i\hat{\omega}\frac{U^*}{d^*} = \sigma\frac{\nu^*}{d^{*2}} \quad \rightarrow \quad \sigma = -i\hat{\omega}\left|\frac{Re_i}{r_i} - \frac{Re_o}{r_o}\right| r_i. \tag{2.7}$$

## 3. Mode structure similarities between high and low Taylor numbers

The flow instability at high Taylor numbers $Ta$ is particularly relevant to accretion disks, for which $Ta$ can reach values estimated to be on the order of $10^{24}$ (Ji et al. 2006; Grossmann et al. 2016). However, achieving such high $Ta$ flows experimentally or numerically is currently unfeasible. To address this challenge, one approach is to investigate potential flow similarities between high $Ta$ and low $Ta$ regimes. Fortunately, we have observed such similarities in the linear framework, as illustrated in figure 3 of the main paper, figures 1 and 2 in this document. These figures depict the eigenvectors of the disturbance of the most unstable axisymmetric and helical modes for $Ta = (10^6, 10^8, 10^{10})$. Notably, these patterns exhibits robust similarities, primarily differing in length scales. We confirm that similar flow patterns persist even at $Ta = 10^{16}$, though the corresponding length scale is much smaller. More specifically, as $Ta$ increases, disturbances become more localised around the inner rotating cylinder. These findings may be pertinent to accretion disk dynamics discussed in the main text in subsection 4.1 of the main paper.

## 4. Mode patterns of the linear instabilities at high azimuthal wavenumbers

In the present study, our focus has primarily been on the axisymmetric mode $m = 0$ and the first few non-axisymmetric modes $m = 1, 2$, as these modes consistently emerge at the

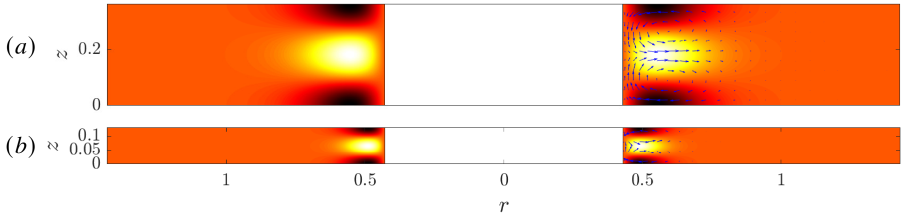


Figure 1: Contours of the temperature corresponding to the most unstable mode disturbance in the quasi-Keplerian flow at $\eta = 0.3$, $Pr = 0.7$ and $Ri = 0.1$. Panel $(a)$ is for the case at $k \approx 17.21$, $m = 0$ and $Ta = 10^8$. Panel $(b)$ is for the case at $k \approx 47.62$, $m = 0$ and $Ta = 10^{10}$. Arrows visualise the velocity vector field.

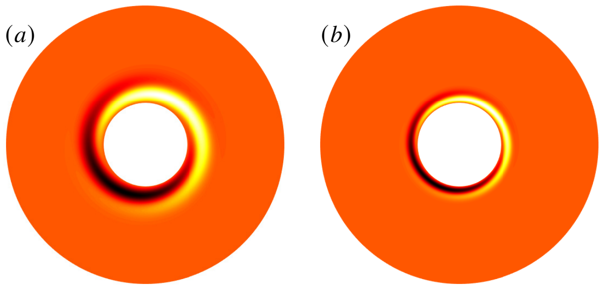


Figure 2: Contours of temperature corresponding to the most unstable non-axisymmetric mode disturbance in the quasi-Keplerian flow at $\eta = 0.3$, $Pr = 0.7$ and $Ri = 0.1$. Panel $(a)$ is for the case at $k \approx 19.81$, $m = 1$ and $Ta = 10^8$. Panel $(b)$ is for the case at $k \approx 55.03$, $m = 1$ and $Ta = 10^{10}$.

critical conditions for the linear instability. However, it is important to note that thermally-driven linear instability can occur at much higher azimuthal wavenumbers as well. This phenomenon is illustrated in figure 4 of the main paper. Remarkably, at $(q, \eta, Pr, Ri, Ta) = (1.5, 0.3, 0.7, 0.1, 10^{10})$, up to 83 non-axisymmetric modes are found to be unstable. The flow structures of these modes at selected parameters are depicted in figure 3. The azimuthal wavenumber $m$ corresponds to a radian period of $2\pi/m$ in the azimuthal direction, indicating the number of distorted counter-rotating vortex pairs aligned azimuthally. As $m$ increases, more convective rolls develop with a reduction in the length scale of these structures. It is noteworthy that disturbances tend to localise away from the inner cylinder wall, resulting in an area near the inner region devoid of disturbances. This localisation around the outer rotating cylinder suggests that these modes may not be relevant to accretion disk dynamics. This is because observations indicate that thermal convection is unlikely to occur in outer disk regions (Latter 2016). Indeed, the convective overstability discovered by Klahr & Hubbard (2014) was found to probably only appear in inner regions of accretion disks (Latter 2016).

## 5. Linear instability in an extreme case at $(\eta, Pr, Ri)$=$(0.05, 10^{-7}, 10^{-7})$

In Section 4 of the main paper, we have demonstrated the prevalence of the linear instability across a broad parameter space covering $O(0.01) \leqslant \eta \leqslant O(0.1)$, $O(10^{-4}) \leqslant Pr \leqslant O(10)$, and $O(10^{-3}) \leqslant Ri \leqslant O(1)$. Regarding the relevance of these parameters to accretion disks, Latter (2016) noted that $Pr$ could be as low as $10^{-7}$ in certain inner radii regions of accretion disks, and $Ri$ is generally much smaller than 1. In this appendix, we explore the persistence

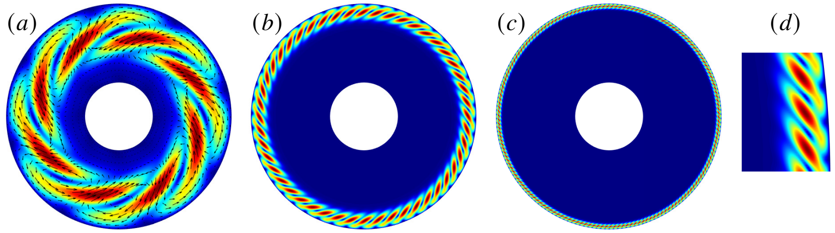


Figure 3: Contours of velocity magnitude corresponding to different non-axisymmetric mode disturbances in the quasi-Keplerian flow at $\eta = 0.3$, $Pr = 0.7$ and $Ri = 0.1$. Panel $(a)$ is for $(Ta, m, k) = (10^6, 4, 2.287)$. Panel $(b)$ is for $(Ta, m, k) = (10^8, 24, 0)$. Panel $(c)$ is for $(Ta, m, k) = (10^{10}, 83, 0)$ and panel $(d)$ shows an enlarged view of panel $(c)$ around its right edge. The mode in panel $(a)$ is axial-dependent ($k \neq 0$) and the figure shown here is the $r$-$\theta$ plane data at axial location $z = 0$.

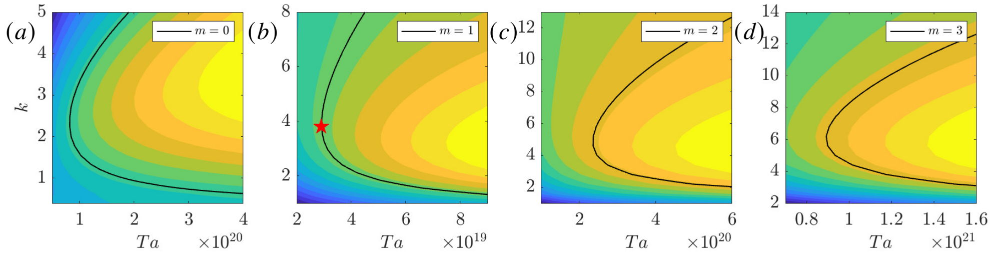


Figure 4: Contours of the linear growth rate $\omega_i$ in the $Ta$-$k$ plane for the quasi-Keplerian flow at $\eta = 0.05$, $Pr = 10^{-7}$, $Ri = 10^{-7}$: from left to right the panels are for $m = 0, 1, 2, 3$, respectively. The black curves are the neutral curves ($\omega_i = 0$). The linear critical condition is attained at about $(Ta_c, k_c, m_c) = (3 \times 10^{19}, 4, 1)$, marked by the red star in panel $(b)$.

of linear instability at the extreme parameter setting of $(\eta, Pr, Ri) = (0.05, 10^{-7}, 10^{-7})$ when the Taylor number is raised to a high level of $Ta = O(10^{19})$. To achieve numerical convergence, the highest spatial resolution used in the present case is $N = 601$.

Figure 4 depicts the corresponding neutral curves near the instability onset. The linear critical condition is observed around $(Ta_c, k_c, m_c) = (3 \times 10^{19}, 4, 1)$, identifying the first helical mode similar to that shown in figure 13 of the main paper for $(\eta, Pr, Ri) = (0.05, 10^{-3}, 10^{-3})$. The mode patterns at four critical points identified in figure 4 are visualised in figure 5. These structures exhibit similarities to those in figure 14 of the main paper for $(\eta, Pr, Ri) = (0.05, 10^{-3}, 10^{-3})$.Two main differences are noticeable. Firstly, the axisymmetric mode becomes more localised around the inner rotating cylinder, and the vortices appear less inclined along the axial $z$ direction. The eigenvalues for this complex-conjugate pair are $\pm 0.309518053476 - 0.000000000006i$, indicating that these two modes propagate axially. An enlarged view of the perturbation field around the inner cylinder does reveal inclined vortices (not shown here). Secondly, the non-axisymmetric modes appear less distorted by the circular base flow, lacking the pronounced "spiral structures" seen in figure 14$(b)$ of the main paper. We infer that these "spiral structures" may exist only within an extremely thin layer adjacent to the boundaries. When examining the modes $m = 1, 2, 3$ in figure 5, one might initially think that the no-slip boundary condition is not being met. To clarify, we have examined the implementation of the no-slip boundary condition and can confirm that there is an extremely sharp gradient in the velocity field near the cylinder

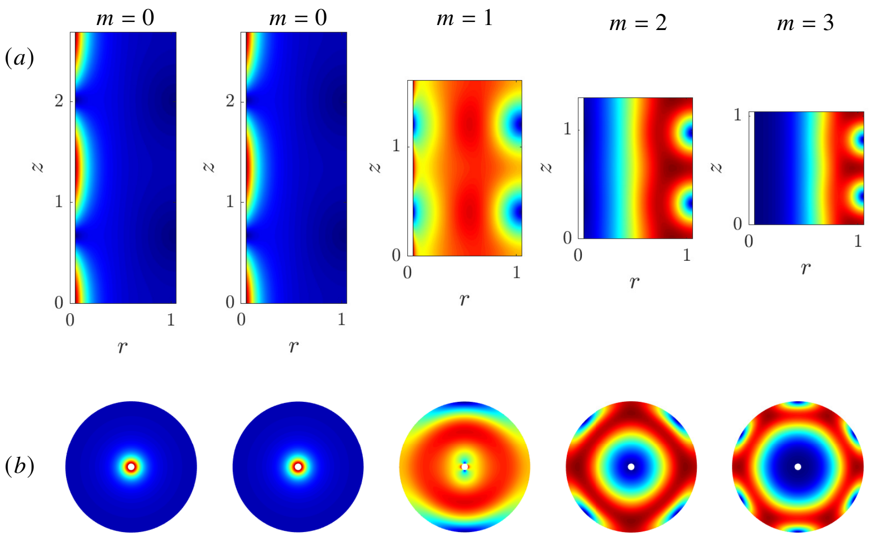


Figure 5: Contours of the perturbation velocity magnitude at the four critical points identified in figure 4. Panel $(a)$ shows the cross sections in the $r$-$z$ plane at the azimuthal angle $\theta = 0$; panel $(b)$ shows the cross sections in the $r$-$\theta$ plane at the axial position $z = 0$. From left to right, the first and second panels in each row correspond to a pair of complex conjugate modes at $m = 0$, the third to fifth panels are for $m = 1, 2, 3$, respectively.

walls at this high $Ta$, ensuring that the no-slip boundary condition is indeed satisfied at the boundary.

## REFERENCES


Deguchi, K. 2017 Linear instability in Rayleigh-stable Taylor-Couette flow. *Phys. Rev. E* **95** (2), 021102.

Grossmann, S., Lohse, D. & Sun, C. 2016 High–Reynolds number Taylor-Couette turbulence. *Annu. Rev. Fluid Mech.* **48**, 53–80.

Ji, H., Burin, M., Schartman, E. & Goodman, J. 2006 Hydrodynamic turbulence cannot transport angular momentum effectively in astrophysical disks. *Nature* **444** (7117), 343–346.

Klahr, H. & Hubbard, A. 2014 Convective overstability in radially stratified accretion disks under thermal relaxation. *Astrophys. J.* **788** (1), 21.

Latter, H.N. 2016 On the convective overstability in protoplanetary discs. *Mon. Not. R. Astron. Soc.* **455** (3), 2608–2618.
